# Supplementary material for: PARS: Pseudo-Label Aware Robust Sample Selection for Learning with Noisy Labels
Source: arXiv:2201.10836 source file (2022-01-26)
Supplement: Supplementary file 1 [file appendix.tex]

\subsection{Open Questions ??}
\begin{enumerate}
    \item Do you think the setting with \textbf{4000 labels and 50\% noise} is similar to \textbf{2000 clean labels} ? Thoughts - maybe not, because we do not have to collect ``clean'' labels to begin with as input to the model. 
    \item For the student teacher framework, we are pushing forward a setting where pseudo labeling/self-training (entropy minimization) works better than consistency regularization? 
    \item Meta-Pseudo Labels paper (\url{https://arxiv.org/pdf/2003.10580.pdf}), they are somewhat proposing a similar student-teacher framework? Have to go in details. 
    \item Some directions could be - a) As the pseudo-labels are highly confident predictions (assumption - they should be more or less clean), so train the student model with a cross-entropy loss than the noise robust loss.
    
    b). Employ a sample selection approach on the pseudo-labels from the unlabeled set to divide them into clean and noisy samples and use only the clean ones in the student framework? 
    
    c). Currently there is no communication between the teacher and the student, so the teacher's responsibility is not to improve the student? Maybe enforcing this in the teacher and having a feedback might help? 
    
    d). Noisy self training has shown to outperform, so maybe look at some works on how to improve self training? 
\end{enumerate}

\section{Results}

\noindent
\textbf{Student-Teacher Loss plots}

\begin{figure}
\begin{center}
\includegraphics[width=\textwidth]{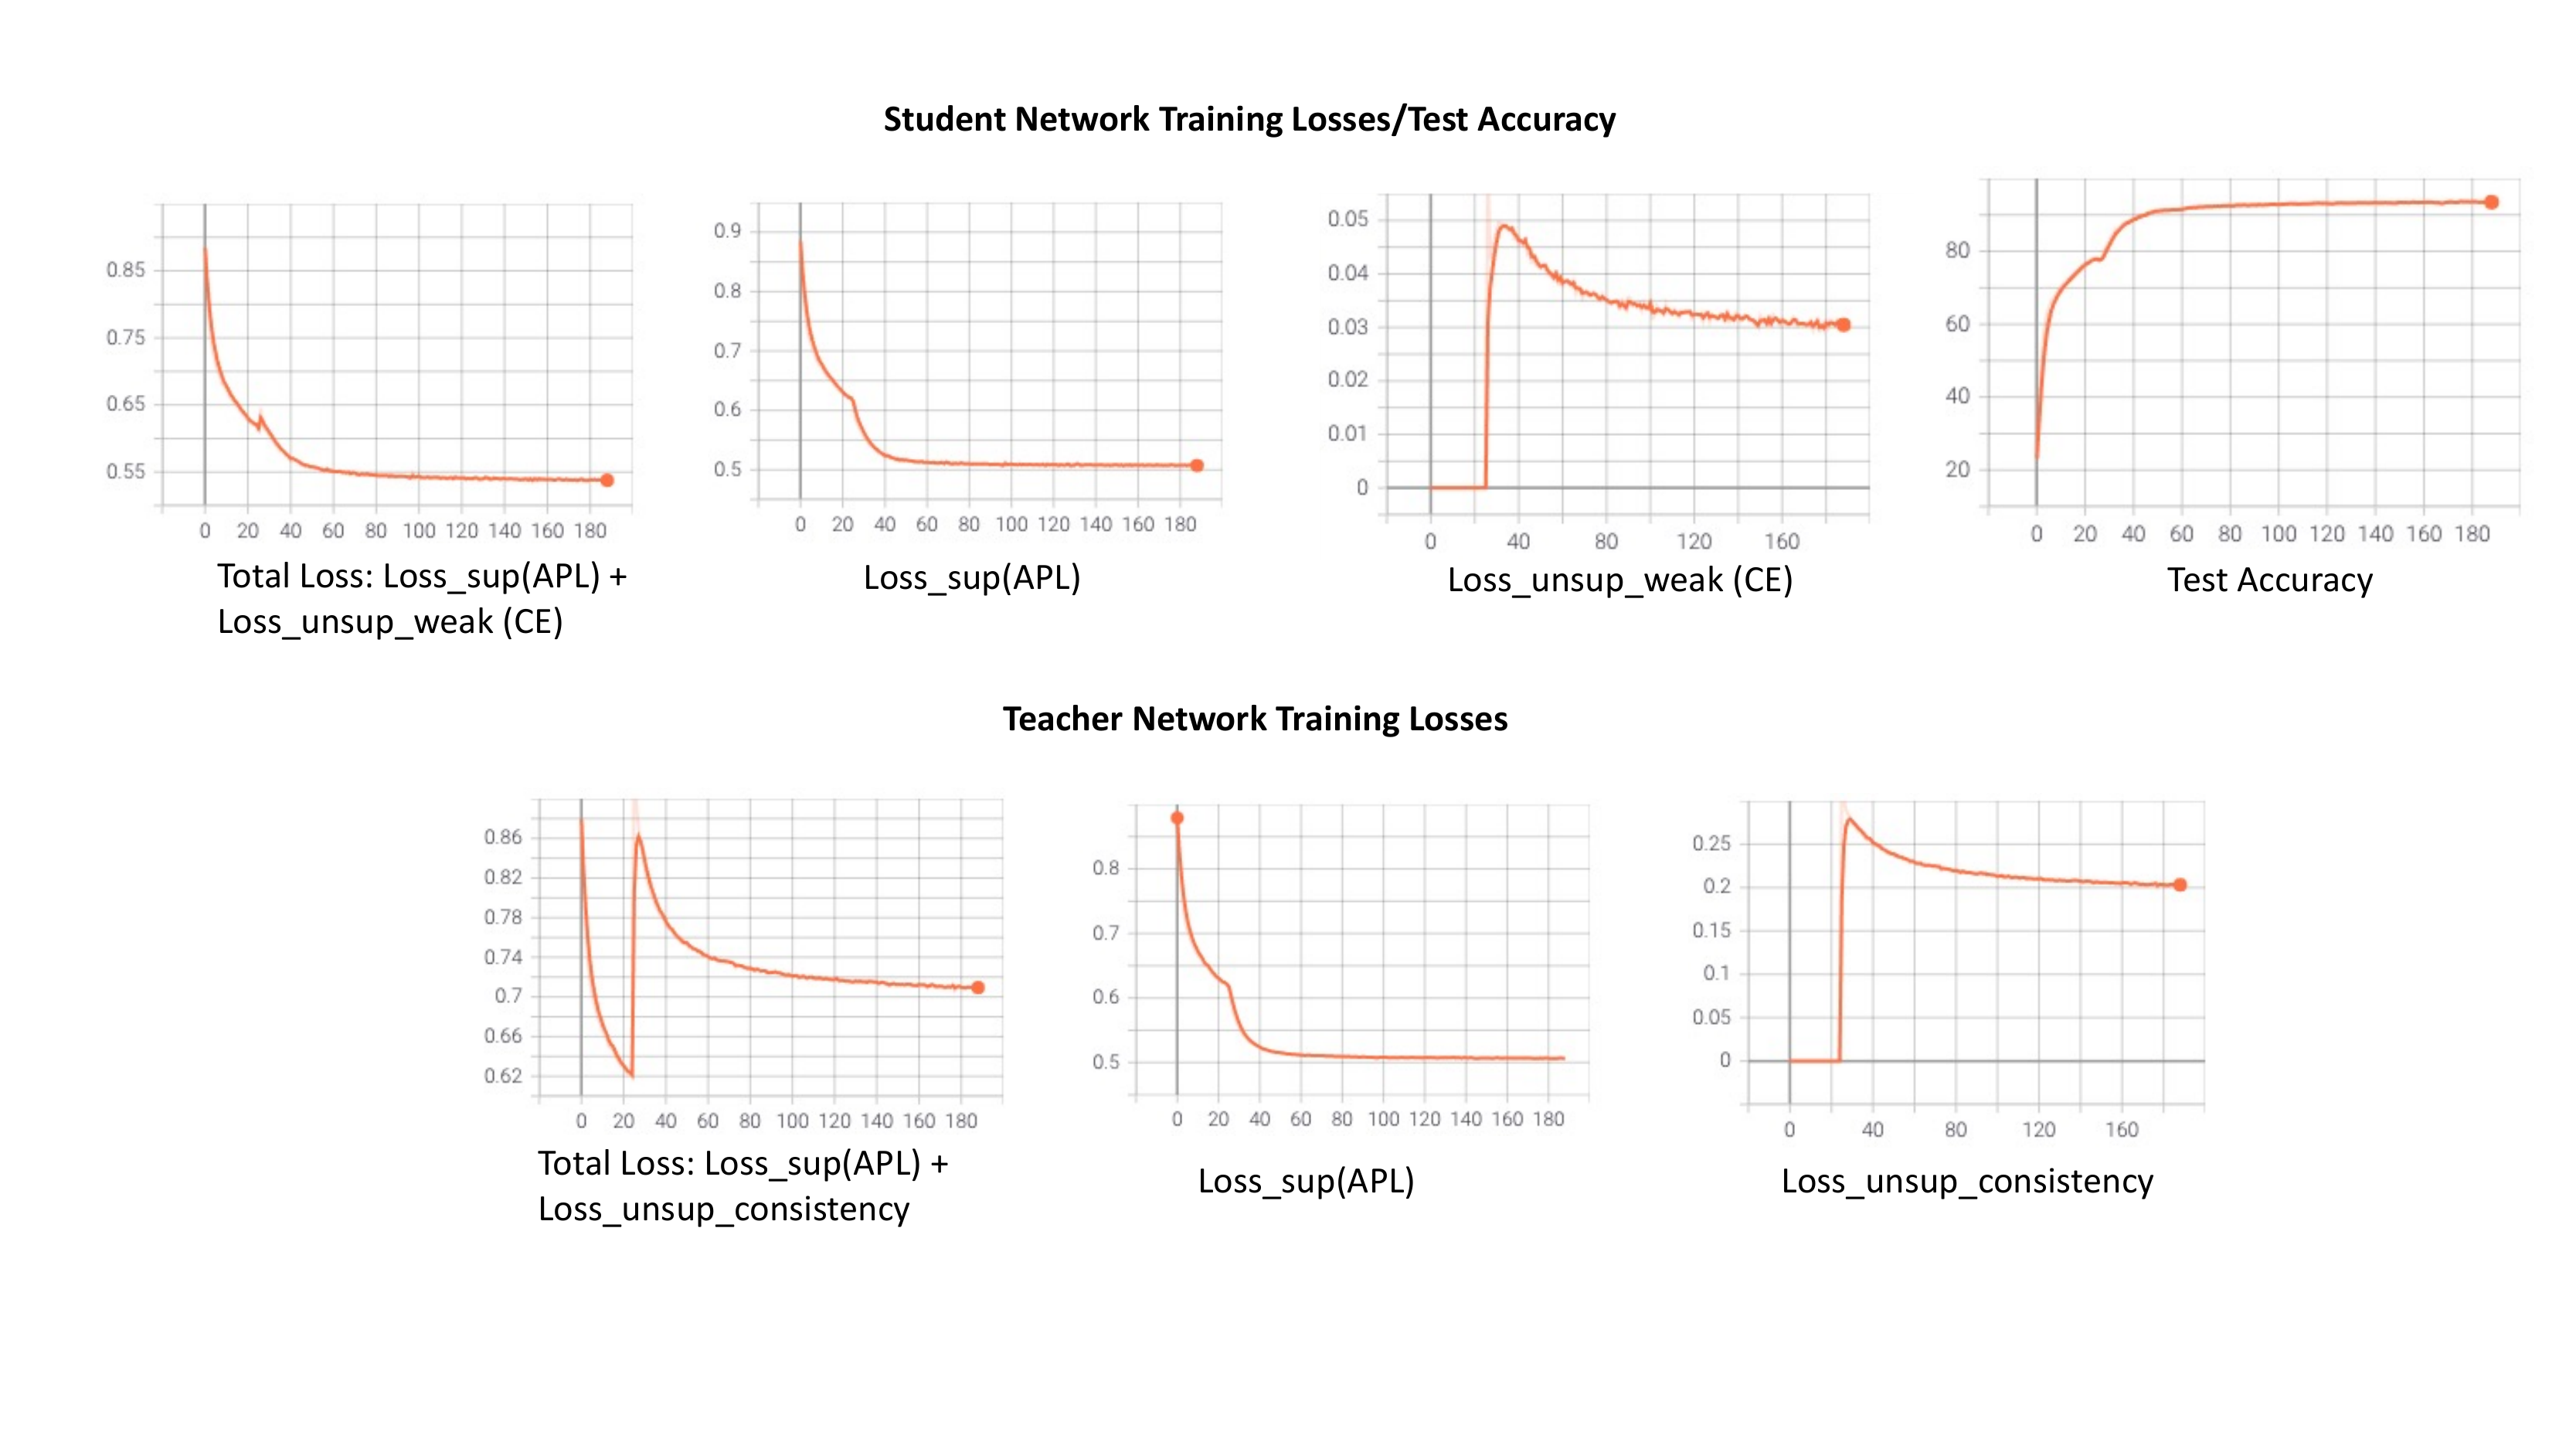}
% \vspace{-.3cm}
\end{center}
\caption{}
\label{fig:loss_stu_tea}
\end{figure}

 \begin{algorithm}
   \caption{Baseline: FixMatch with WarmUp Training}
    \begin{algorithmic}[1]
        \State \textbf{Input: } Noisy labeled dataset $\mathcal{D}_{L} = \{{(\bm{x}_l,y_l)}^{(i)}\}{_{i=1}^{n_l}}$, unlabeled examples $\mathcal{D_U} = \{{(\bm{x}_u)}^{(i)}\}{_{i=1}^{n_u}}$, confidence threshold $\tau$, unlabeled loss weight $\lambda_u$, $\alpha$ and $\mathcal{A}$ are weak and strong augmentation func. respectively for FixMatch, total epochs $E$, WarmUp epoch $w_e$ ($w_e$ < $E$) and model parameters $\theta$. 
        \While{$e$ < $w_e$}
            \State $\hat{p}_l$ = $p_{model}(\bm{x}_l; \theta)$
            \State $L_{x} = \frac{1}{n_l} \sum{_{i=1}^{n_l}} L_{NRL}(\hat{p}_l^i, y_l^i)$ \Comment{\small{\texttt{Warmup  training on the noisy labeled set using Noise Robust Loss (NRL)}}}
        \EndWhile
        
        \State \texttt{// Adding consistency loss for unlabeled examples after warmup}
        % \State $l_{s_{tea}} = \frac{1}{n_u} \sum{_{b=1}^B} H(p_b, \alpha^*(x_b))$ \Comment{\textit{Cross Entropy for labeled data}}
        \For{$e = w_e$ to $E$}
        \For{$i = 1$ to $n_u$}
            \State $\hat{p}_u^i = p_{model}(\alpha(x_u^i); \theta)$ \Comment{\small{\texttt{Compute prediction after applying weak aug. to $x_u$}}}
        \EndFor
        
        \State $L_u = \frac{1}{n_u} \sum{_{i=1}^{n_u}} \{max(\hat{p}_u^i) > \tau\} L_{sup}(p_{model}(\mathcal{A}(x_u^i); \theta), \argmax(\hat{p}_u^i)))$ \Comment{\texttt{Supervised Loss between weak aug. pseudo-label and prediction on strong aug.}}
        \EndFor
        \State \textbf{return} $L_{x} + \lambda_u.L_{u}$

\end{algorithmic}
\label{algo:fixmatch_noisy_baseline}
\end{algorithm}

 \begin{algorithm}
   \caption{Naive Way//FixMatch with Noisy Labels v1.0}
    \begin{algorithmic}[1]
        \State \textbf{Input: } Noisy/Weak Labeled batch $\mathcal{X}$ = $\{(x_b, p_b) : b \in (1, \ldots, B) \}$, unlabeled batch $\mathcal{U}$ = $\{u_b : b \in (1, \ldots, \mu B) \}$, confidence threshold $\tau$, unlabeled data ratio $\mu$, unlabeled loss weight $\lambda_u$

        \State $l_{stu} = \frac{1}{B} (\sum{_{b=1}^B} L_{nce}(p_b, \alpha(x_b)) + \sum{_{b=1}^B} L_{mae}(p_b, \alpha(x_b))$ \Comment{\textit{Warmup student training with noise robust Normalized Cross Entropy (NCE) and Mean Absolute Error (MAE) loss}}
      
        \For{$b = 1$ to $\mu B$}
            \State $q_b = p_m(y | \alpha(u_b); \theta)$ \Comment{\textit{Compute prediction after applying weak data aug of $u_b$}}
        \EndFor
        
        \State $l_u = \frac{1}{\mu B} \sum{_{b=1}^{\mu B}} \{max(q_b) > \tau\} H(\argmax(q_b), p_m(y | \mathcal{A}(u_b)))$ \Comment{\textit{Cross Entropy Loss with pseudo-label and confidence for unlabeled data}}
        \State \textbf{return} $l_{stu} + \lambda_u l_u$

\end{algorithmic}
\label{algo:fixmatch_noisy1.0}
\end{algorithm}

\begin{algorithm}
   \caption{PAWS: \textbf{P}seudo-Label \textbf{A}ware \textbf{W}eak \textbf{S}tudent}
    \begin{algorithmic}[1]
        \State \textbf{Input: } Noisy labeled dataset $\mathcal{D}_{L} = \{{(\bm{x}_l,y_l)}^{(i)}\}{_{i=1}^{n_l}}$, unlabeled examples $\mathcal{D_U} = \{{(\bm{x}_u)}^{(i)}\}{_{i=1}^{n_u}}$, confidence threshold $\tau$, unlabeled loss weight $\lambda_u$,negative learning loss weight $\lambda_n$, $\alpha$ and $\mathcal{A}$ are weak and strong augmentation func. respectively for FixMatch, total epochs $E$, WarmUp epoch $w_e$ ($w_e$ < $E$), student model parameters $\theta_s$ and teacher model parameters $\theta_t$. 
        \While{$e$ < $w_e$}
            \State $\hat{s}_l$ = $s_{model}(\bm{x}_l; \theta_s)$
            \State $\hat{t}_l$ = $t_{model}(\bm{x}_l; \theta_t)$
            \State $L_{s_{x}} = \frac{1}{n_l} \sum{_{i=1}^{n_l}} L_{NRL}(\hat{s}_l^i, y_l^i)$ \Comment{\small{\texttt{Student model Warmup training on the noisy labeled set using Noise Robust Loss (NRL)}}}
            \State $L_{t_{x}} = \frac{1}{n_l} \sum{_{i=1}^{n_l}} L_{NRL}(\hat{t}_l^i, y_l^i)$ \Comment{\small{\texttt{Teacher model Warmup training on the noisy labeled set using Noise Robust Loss (NRL)}}}
        \EndWhile
        
        \State \texttt{// Alternative to Student and Teacher Individual WarmUp}
        \While{$e$ < $w_e$}
            \State $\hat{t}_l$ = $t_{model}(\bm{x}_l; \theta_t)$
            \State $L_{t_{x}} = \frac{1}{n_l} \sum{_{i=1}^{n_l}} L_{NRL}(\hat{t}_l^i, y_l^i)$ \Comment{\small{\texttt{Teacher model Warmup training on the noisy labeled set using Noise Robust Loss (NRL)}}}
        \EndWhile
        \State $\theta_s := \theta_t$ \Comment{\small{\texttt{Assign teacher model's warmup parameters to the student model}}}
        \State \texttt{// Adding consistency loss to Teacher model for unlabeled examples after warmup}
        % \State $l_{s_{tea}} = \frac{1}{n_u} \sum{_{b=1}^B} H(p_b, \alpha^*(x_b))$ \Comment{\textit{Cross Entropy for labeled data}}
        \For{$e = w_e$ to $E$}
        \For{$i = 1$ to $n_u$}
            \State $\hat{t}_u^i = t_{model}(\alpha(x_u^i); \theta_t)$ \Comment{\small{\texttt{Compute prediction after applying weak aug. to $x_u$}}}
        \EndFor
        
        \State $L_{t_{u}} = \frac{1}{n_u} \sum{_{i=1}^{n_u}} \{max(\hat{t}_u^i) > \tau\} L_{sup}(t_{model}(\mathcal{A}(x_u^i); \theta_t), \argmax(\hat{t}_u^i)))$ \Comment{\texttt{Supervised Loss between weak aug. pseudo-label and prediction on strong aug.}}
        \State $L_t = L_{t_{x}} + \lambda_u.L_{t_{u}}$   \Comment{\texttt{Combined Teacher Loss}}
        \State \texttt{// Augment labeled set with pseudo-labeled data from teacher for supervised student training}
        \State $L_{s_{p}} = \frac{1}{n_u} \sum{_{i=1}^{n_u}} \{max(\hat{t}_u^i) > \tau\} [ L_{PL}(s_{model}([\mathcal{A}(x_u^i),\alpha(x_u^i)]; \theta_t), \argmax(\hat{t}_u^i)))$  \Comment{\texttt{Positive Learning Loss for pseudo-labeled samples above threshold}}
        \State $L_{s_{n}} = \frac{1}{n_u} \sum{_{i=1}^{n_u}} \{max(\hat{t}_u^i) < \tau\} [ L_{NL}(s_{model}([\mathcal{A}(x_u^i),\alpha(x_u^i)]; \theta_t), \argmax(\hat{t}_u^i)))$ \Comment{\texttt{Negative Learning Loss for pseudo-labeled samples below threshold}}
        \State $L_s = L_{s_{x}} + L_{s_{p}} + \lambda_n. L_{s_{n}}$   \Comment{\texttt{Combined Student Loss}}
        \EndFor
        \State \textbf{return} $L_t, L_s$

\end{algorithmic}
\label{algo:paws}
\end{algorithm}

 \begin{algorithm}
   \caption{FixMatch with Noisy Labels v1.1 // Student and Teacher model are different}
    \begin{algorithmic}[1]
        \State \textbf{Input: } Noisy/Weak Labeled batch $\mathcal{X}$ = $\{(x_b, p_b) : b \in (1, \ldots, B) \}$, unlabeled batch $\mathcal{U}$ = $\{u_b : b \in (1, \ldots, \mu B) \}$, confidence threshold $\tau$, unlabeled data ratio $\mu$, unlabeled loss weight $\lambda_u$, epoch $e$

        \State $l_{stu} = \frac{1}{B} (\sum{_{b=1}^B} L_{nce}(p_b, \alpha(x_b)) + \sum{_{b=1}^B} L_{mae}(p_b, \alpha(x_b))$ \Comment{\textit{Warmup student training with noise robust Normalized Cross Entropy (NCE) and Mean Absolute Error (MAE) loss}}
        \State Train a teacher model in a semi-supervised way using the Fix-Match approach. 
        \State $l_{s_{tea}} = \frac{1}{B} \sum{_{b=1}^B} H(p_b, \alpha^*(x_b))$ \Comment{\textit{Cross Entropy for labeled data}}
      
        \For{$b = 1$ to $\mu B$}
            \State $q_b = p_m(y | \alpha^*(u_b); \theta^*)$ \Comment{\textit{Compute prediction after applying weak data aug of $u_b$}}
        \EndFor
        
        \State $l_{u_{tea}} = \frac{1}{\mu B} \sum{_{b=1}^{\mu B}} \{max(q_b) > \tau\} H(\argmax(q_b), p_m(y | \mathcal{A}(u_b)))$ \Comment{\textit{Cross Entropy Loss with pseudo-label and confidence for unlabeled data}}
        \State $l_{tea} = l_{s_{tea}} + \lambda_u l_{u_{tea}}$
        \State Augment student training set with pseudo-labeled data above threshold $\tau$, $(u_b, q_b)$ to compute $l_{stu}$ with $(x_b, p_b)$ and $(u_b, q_b)$. 
        \State \textbf{return} $l_{stu} + l_{tea}$

\end{algorithmic}
\label{algo:fixmatch_noisy1.1}
\end{algorithm}

\begin{enumerate}

 \item \textbf{\Cref{algo:fixmatch_noisy1.0} - A small set of noisy labeled samples with unlabeled samples in a FixMatch setting.}

In our setting of semi-weak supervision, we assume that our labeled set is not perfectly clean and has some label noise, unlike in existing approaches. The unlabeled set is formulated and exploited during training in the same way as traditional semi-supervised learning approaches. 

\textbf{What we expect from such a setting? \arushi{[WIP]}} Firstly, it reduces the overhead of collecting a clean labeled set and depends on labels collected via noisy sources (a mixture of clean and noisy data). Secondly, the noise in the labeled samples can be a helpful tool during training as the model is more robust to noise, which will help in predicting confident pseudo-labels for more unlabeled samples. \arushi{Does it make sense to say that we need very few clean labels?? Even with 90\% noise there are few clean labels. Or another way to formulate is we take advantage of noise in the labels along with unlabeled samples to improve training. Also, there are a few methods that exploit this large scale weakly labeled data during training, but the collection of these is also expensive and can we argue that training on noisy and unlabeled is better than just training on all noisy labels. Can we theoretically formulate this?}

In \Cref{algo:fixmatch_noisy1.0}, we first train a noise robust loss function \cite{ma2020normalized} on the labeled samples (line 2) and then add the unsupervised consistency loss, $l_u$, by predicting pseudo-targets for the weakly augmented data which are the pseudo ground-truth labels for the strongly augmented version of the samples, as in the FixMatch setup.  

A few ablations could be - 1). Testing the accuracy of the model only with warmup training without adding unlabeled samples, 2). Not treating all the unlabeled samples as equal, using the noisy labels for some of them during training based on some learned weights (\arushi{WIP}).

% Does it make sense to say that we need very few clean labels?? Even with 90% noise there are few clean labels. Or another way to formulate is we take advantage of noise in the labels along with unlabeled samples to improve training. There are a few methods that exploit this large scale weakly labeled data during training, but the collection of these is also expensive and we argue that 

\item 
\textbf{\Cref{algo:fixmatch_noisy1.1} - Self-training with unlabeled examples in a student-teacher model framework.}

In \Cref{algo:fixmatch_noisy1.1}, we discuss our student-teacher framework for learning with noisy and unlabeled samples. The input to the student model are the noisy labeled examples and the student model goes through warmup training using a noise robust loss (line 2). We have another teacher model similar to the student model that takes as input the noisy labeled samples and the unlabeled samples. The teacher model is trained in the same way as FixMatch (lines 3-9). The student model is then augmented with the pseudo-labels predicted from the teacher model for the unlabeled samples and the student training continues with the loss in line 2. Both the student and teacher model parameters are trained together (line 11). 

Why a student-teacher model framework better? \arushi{WIP}

where $p_c$ denotes the prior probability distribution for class $c$ and $\bar{h}_{{stu}_c}$ and $\bar{h}_{{tea}_c}$ are the mean softmax probability of the student and teacher models respectively for class $c$ across all labeled and unlabeled samples in the mini-batch.

\noindent
\textbf{-- Loss Functions for less confident pseudo-labeled data (threshold < 0.95)} 
For these low confident samples, we do not want to use the hard pseudo labels from the teacher network as they might be wrong and hence lead to poor performance of the student network. But we do not want to ignore/discard these samples as well, as they might have some important training signal that can be useful for student model's convergence. 

Hence, it is very important to chose a loss function and a weight for this loss that such that the model neither completely ignores these samples but learn something from them in a softer way. 
Some naive loss functions to try are - 1) CE Loss, 2) Noise Robust Loss (Active+Passive Loss (APL), 3) Mean Squared Error (Tried, but does not make sense to use this), 4) KL-Divergence/ JS-Divergence, 5) Label Smoothing Regularization.

\textbf{Negative Cross Entropy \cite{kim2019nlnl}} Inspired by negative learning in \cite{kim2019nlnl}, we treat all the pseudo-labels below a certain threshold (0.95 in this case) as complementary/wrong labels, $\bar{y_k}$. Unlike the standard CE loss training where we optimize the probability value corresponding to the given (true) label to be close to 1, in negative learning (NL) we instead optimize the output probability corresponding to the complementary/wrong label to be far from 1 (to reach 0). The loss function that supports this objective is formulated as - 

\begin{equation}
    L_{pl < \tau}(f, \bar{y}) = - \sum_{k=1}^C \bar{y_k} log(1 - p_k)
\end{equation}

The gradient for the above loss is given as - 
\begin{equation}
  \frac{\partial L_{pl < \tau}(f, \bar{y})}{\partial f_i} =
    \begin{cases}
      \bm{p_i} \approx \frac{1}{c} & \text{if $i$ = $\bar{y}$}\\
      - \frac{\bm{p_{\bar{y}}}}{1 - \bm{p_{\bar{y}}}} \bm{p_i} & \text{if $i \neq \bar{y}$}
      
    \end{cases}       
\end{equation}

\arushi{Is there something we can say wrt to the gradient for this loss function? Is it able to provide good gradient and hence preventing the model to overfit by not providing wrong information?}

\arushi{The accuracy of the pseudo-labels on the unlabeled data from the teacher network are - Top 1 Accuracy: 52.66\% and Top 5 Accuracy - 74.49\%. The top-1 accuracy on the clean set of pseudo labels (>threshold) is 53.79\% and top-5 accuracy is 74.54\%. The top-1 accuracy on the noisy set of pseudo labels (<threshold) is 30.95\% and top-5 accuracy is 73.81\%.}

\noindent
\textbf{Entropy Distributions for Clean and Noisy Labels}

\textbf{Tsne of feature representations from the final model vs baselines} 

\textbf{Performance on samples selected data, how does it reduce noise ratio compared to original data}

\noindent
\textbf{\Cref{table:sota_ssl}: Small Noisy Labeled Set (with 50 \% noise) + Unlabeled Data}

\noindent
\textbf{Baselines. }

1). \textbf{FixMatch \cite{sohn2020fixmatch}} - We report results from the original FixMatch paper which is trained on the traditional semi-supervised learning setting with a subset of clean labels and a large unlabeled training set. \textbf{Please note in this case there is no noise in the labeled set.  }

2).\textbf{ FixMatch (Retrain)} - We retrain the FixMatch algorithm on our setting with a small noisy labeled set and a large unlabeled set. In the original FixMatch setting, there is no ``warmup'' training for the labeled set and the unsupervised loss gets active when the pseudo-labels get above a certain threshold (0.95). Following this approach fails for our setting as the model predicts wrong overconfident pseudo-labels in the initial epochs which hurt the overall training. To prevent this, we introduce a forced warmup training on the noisy labeled set for a few epochs (50 epochs) and then add the unsupervised objective as in FixMatch.  

3). \textbf{DivideMix \cite{li2020dividemix}} - In DivideMix, they begin with a large noisy labeled set and then select clean and noisy samples based on a sample selection approach. Then, they treat the clean labels as a (strongly) labeled set and the noisy labels as the unlabeled set and train the model in a semi-supervised way. 

We retrain DivideMix on our setting of a small noisy labeled set and a pre-known unlabeled set. In detail, the sample selection approach divides the small noisy labeled samples (for instance, 4000 labels) to a clean and a noisy set, where these noisy labels are added to the pre-existing unlabeled set. 

\noindent
\textbf{Proposed Method, Algorithm 2. }

1). \textbf{Alg. 2, Warmup stage: APL Loss (Ours)} - We train the small noisy labeled set (for instance, 4000 labels with 50\% noise) with the noise robust loss functions, Active Passive Losses (APL) \cite{ma2020normalized} until convergence (80 epochs) without any unlabeled samples. This helps to give a good baseline for our algorithm and to measure the performance difference when the model is trained with unlabeled samples. 

2). \textbf{Alg. 2, Warmup stage-APL + FixMatch (Ours)} - This is our final model proposed in \Cref{algo:fixmatch_noisy1.0} with an initial warmup training (40 epochs) using the APL loss on the small noisy labels and then adding the unsupervised objective following the FixMatch algorithm.

\noindent
\textbf{\Cref{table:sota_noisy}: Large Noisy Labeled Set + Weakly Augmented Unlabeled Data}

When there is high noise (90\%), the model overfits to the noise when trained with very few samples. Hence, we propose to keep the entire noisy dataset and use the augmented versions of the images as the unlabeled dataset to regulate the noisy supervision training.  

\noindent
\textbf{Proposed Method, Algorithm 3. - Student Teacher Framework}

1). \textbf{Alg. 3, Student-Teacher Model (Ours)} - In this model, we first do initial warmup for both the student and teacher models (no shared parameters) using noise robust losses. After this warmup, we add the unsupervised loss to the teacher model and predict pseudo-labels for the unlabeled data. If the predictions on the unlabeled data are above a certain threshold, we add these samples to the student training batch and train the augmented student with the noise robust loss function. Both the student and teacher models are trained simultaneously until convergence.

\noindent
\textbf{-- Self training of the Student model with noisy pseudo labeled data (threshold < 0.95)}

\noindent
\textbf{-- Augmentations on the Unlabeled data for Student Training : Horizontal Flip, CutOut and CutMix}

\noindent
\textbf{-- Dynamic Threshold for Pseudo-Labels in the Student Network}

\noindent
\textbf{-- Label Co-Guessing for weakly and strongly augmented unlabeled data while training teacher network. }

%  \begin{algorithm}
%   \caption{FixMatch with Noisy Labels v1.1 // Student and Teacher model are the same}
%     \begin{algorithmic}[1]
%         \State \textbf{Input: } Noisy/Weak Labeled batch $\mathcal{X}$ = $\{(x_b, p_b) : b \in (1, \ldots, B) \}$, unlabeled batch $\mathcal{U}$ = $\{u_b : b \in (1, \ldots, \mu B) \}$, confidence threshold $\tau$, unlabeled data ratio $\mu$, unlabeled loss weight $\lambda_u$, epoch $e$

%         \State $l_{stu} = \frac{1}{B} (\sum{_{b=1}^B} L_{nce}(p_b, \alpha(x_b)) + \sum{_{b=1}^B} L_{mae}(p_b, \alpha(x_b))$ \Comment{\textit{Warmup student training with noise robust Normalized Cross Entropy (NCE) and Mean Absolute Error (MAE) loss}}
      
%         \For{$b = 1$ to $\mu B$}
%             \State $q_b = p_m(y | \alpha(u_b); \theta)$ \Comment{\textit{Compute prediction after applying weak data aug of $u_b$}}
%         \EndFor
        
%         \State $l_u = \frac{1}{\mu B} \sum{_{b=1}^{\mu B}} \{max(q_b) > \tau\} H(\argmax(q_b), p_m(y | \mathcal{A}(u_b)))$ \Comment{\textit{Cross Entropy Loss with pseudo-label and confidence for unlabeled data}}
%         \State Augment student training set with pseudo-labeled data above threshold $\tau$, $(u_b, q_b)$ to compute $l_{stu}$ with $(x_b, p_b)$ and $(u_b, q_b)$. 
%         \State \textbf{return} $l_{stu} + \lambda_u l_u$

% \end{algorithmic}
% \end{algorithm}

% \item 
% Algorithm 4 - (SIGUA + Warmup) for noisy sample selection

\end{enumerate}

\begin{figure}
\begin{center}
\includegraphics[width=\textwidth]{figures/Student-Teacher Model.pdf}
% \vspace{-.3cm}
\end{center}
\caption{}
\label{fig:stu_tea}
\end{figure}

\begin{table*}[t]

% 	\begin{center}
		
		\resizebox{1.0\textwidth}{!}{
			\begin{tabular}{|l | l |c c c c |c c  c|}
				\hline
				Datasets & & \multicolumn{4}{c|}{CIFAR-10} &\multicolumn{3}{c|}{CIFAR-100} \\
				\hline
				\#Labels & &40 & 250 & 4000 & All Labels & 400 & 2500 & 10000 \\ 
				\hline
                FixMatch \cite{sohn2020fixmatch} & & 86.19 & 94.93 & 95.74 &- & 51.15 & 71.71 & 77.40 \\ \hline
                \multirow{8}{*}{50\% Sym. noise} & FixMatch (Retrain) &  &  & 82.69  & &  &  &  \\
                & DivideMix+ \cite{li2020dividemix} (Retrain) &  &  & 74.31 &  &  &  &  \\ \cline{2-9}
                
                & Alg. 2, Warmup stage: APL Loss ({\color{blue}{{Ours}}}) &  &  & 80.21 & &  &  &  \\
	            & Alg. 2, Warmup stage -APL + FixMatch  (Ours) &  &  & 94.93 & 95.32/8000labels & &  &  \\
				& Alg. 2, Warmup stage -APL + Sample Selection + FixMatch  (Ours) &  &  & 95.15 & 96.31* & &  &  \\  \cline{2-9}
                
	            & Alg. 3, Student-Teacher Model (Ours), $L_{{lab}_{APL}} + L_{{un-weak}_{APL}}$ &  &  & 92.64 &  & &  &  \\
	            
	            & Alg. 3, Student-Teacher Model (Ours), $L_{{lab}_{APL}} + L_{{un-weak}_{CE}}$ &  &  & 93.52 &  & &  &  \\
	            & Alg. 3, Student-Teacher Model (Ours), $L_{{lab}_{APL}} + L_{{(un-(weak, strong) > \tau)}_{CE}} $ &  &  & 94.72 &  & &  &  \\
	            
	            & Alg. 3, Student-Teacher Model (Ours), $L_{{lab}_{APL}} + L_{{(un-(weak, strong,cutmixaug) > \tau)}_{CE}}$ &  &  & 95.40 &  & &  &  \\
	            & Alg. 3, Student-Teacher Model (Ours), $L_{{lab}_{APL}} + L_{{(un-(weak, strong,cutmixaug) > \tau)}_{CE}} + 0.1 * L_{{(un-(weak, strong) < \tau)}_{neg-ce}}$ &  &  & 95.67 &  & &  &  \\
	           % & Alg. 3, Student-Teacher Model (Ours), $L_{{lab}_{APL}} + L_{{(un-(weak, strong) > \tau)}_{CE}} + L_{{(un-(weak, strong) < \tau)}_{MSE}}$ &  &  & 95.38 &  & &  &  \\
				\hline
				
				\multirow{9}{*}{90\% Sym. noise} & FixMatch (Retrain) &  &  &  & &  &  &  \\
				& DivideMix \cite{li2020dividemix} &  &  &  & 76.0 &  &  &  \\ 
                & DivideMix+ \cite{li2020dividemix} (Retrain) &  &  &  &  &  &  &  \\ \cline{2-9}
                
                & Alg. 2, Warmup stage: APL Loss ({\color{blue}{{Ours}}}) &  &  & 56.49 & &  &  &  \\
	            & Alg. 2, Warmup stage -APL + FixMatch  (Ours) &  &  & 79.73 &  & &  &  \\ \cline{2-9}

	            & Alg. 3, Student-Teacher Model (Ours), $L_{{lab}_{APL}} + L_{{un-weak}_{APL}}$ &  &  &  &  & &  &  \\
            
	            & Alg. 3, Student-Teacher Model (Ours), $L_{{lab}_{APL}} + L_{{un-weak}_{CE}}$ &  &  & &  & &  &  \\
	            & Alg. 3, Student-Teacher Model (Ours), $L_{{lab}_{APL}} + L_{{(un-(weak, strong) > \tau)}_{APL}} $ &  &  & 80.52 &  & &  &  \\
	            & Alg. 3, Student-Teacher Model (Ours), $L_{{lab}_{APL}} + L_{{(un-(weak, strong) > \tau)}_{APL}} + 0.1 * L_{{(un-(weak, strong) < \tau)}_{neg-ce}}$ &  &  & 81.23 &  & &  &  \\
				\hline
				
                \multirow{9}{*}{40\% Asym. noise} & FixMatch (Retrain) &  &  &  & &  &  &  \\
				& DivideMix \cite{li2020dividemix} &  &  &  & 93.4 &  &  &  \\ 
                & DivideMix+ \cite{li2020dividemix} (Retrain) &  &  &  &  &  &  &  \\ \cline{2-9}
                
                & Alg. 2, Warmup stage: APL Loss ({\color{blue}{{Ours}}}) &  &  &  & &  &  &  \\
	            & Alg. 2, Warmup stage -APL + FixMatch  (Ours) &  &  & 94.03 &  & &  &  \\ \cline{2-9}

	            & Alg. 3, Student-Teacher Model (Ours), $L_{{lab}_{APL}} + L_{{un-weak}_{APL}}$ &  &  &  &  & &  &  \\
            
	            & Alg. 3, Student-Teacher Model (Ours), $L_{{lab}_{APL}} + L_{{un-weak}_{CE}}$ &  &  & &  & &  &  \\
	            & Alg. 3, Student-Teacher Model (Ours), $L_{{lab}_{APL}} + L_{{(un-(weak, strong) > \tau)}_{APL}} $ &  &  &  &  & &  &  \\
	            & Alg. 3, Student-Teacher Model (Ours), $L_{{lab}_{APL}} + L_{{(un-(weak, strong) > \tau)}_{APL}} + 0.1 * L_{{(un-(weak, strong) < \tau)}_{neg-ce}}$ &  &  &  &  & &  &  \\
				\hline
\end{tabular}}
\caption{Performance comparison with SOTA Semi-Supervised Learning methods on CIFAR 10/100.}
\label{table:sota_ssl}
\end{table*}

\begin{table*}[t]

% 	\begin{center}
		
		\resizebox{1.0\textwidth}{!}{
			\begin{tabular}{|l | l |c c c c |c c  c|}
				\hline
				Datasets & & \multicolumn{4}{c|}{CIFAR-10} &\multicolumn{3}{c|}{CIFAR-100} \\
				\hline
				\#Labels & &40 & 250 & 4000 & All Labels & 400 & 2500 & 10000 \\ 
				\hline
                FixMatch \cite{sohn2020fixmatch} & & 86.19 & 94.93 & 95.74 &- & 51.15 & 71.71 & 77.40 \\ \hline
                \multirow{8}{*}{50\% Sym. noise} & FixMatch (Retrain) &  &  & 82.69  & &  &  &  \\
                & DivideMix+ \cite{li2020dividemix} (Retrain) &  &  & 74.31 &  &  &  &  \\ \cline{2-9}
                
                & Alg. 2, Warmup stage: APL Loss ({\color{blue}{{Ours}}}) &  &  & 80.21 & &  &  &  \\
	            & Alg. 2, Warmup stage -APL + FixMatch  (Ours) &  &  & 94.93 & 95.32/8000labels & &  &  \\
				& Alg. 2, Warmup stage -APL + Sample Selection + FixMatch  (Ours) &  &  & 95.15 & 96.31* & &  &  \\  \cline{2-9}
                
	            & Alg. 3, Student-Teacher Model (Ours), $L_{{lab}_{APL}} + L_{{un-weak}_{APL}}$ &  &  & 92.64 &  & &  &  \\
	            
	            & Alg. 3, Student-Teacher Model (Ours), $L_{{lab}_{APL}} + L_{{un-weak}_{CE}}$ &  &  & 93.52 &  & &  &  \\
	            & Alg. 3, Student-Teacher Model (Ours), $L_{{lab}_{APL}} + L_{{(un-(weak, strong) > \tau)}_{CE}} $ &  &  & 94.72 &  & &  &  \\
	            
	            & Alg. 3, Student-Teacher Model (Ours), $L_{{lab}_{APL}} + L_{{(un-(weak, strong,cutmixaug) > \tau)}_{CE}}$ &  &  & 95.40 &  & &  &  \\
	            & Alg. 3, Student-Teacher Model (Ours), $L_{{lab}_{APL}} + L_{{(un-(weak, strong,cutmixaug) > \tau)}_{CE}} + 0.1 * L_{{(un-(weak, strong) < \tau)}_{neg-ce}}$ &  &  & 95.67 &  & &  &  \\
	           % & Alg. 3, Student-Teacher Model (Ours), $L_{{lab}_{APL}} + L_{{(un-(weak, strong) > \tau)}_{CE}} + L_{{(un-(weak, strong) < \tau)}_{MSE}}$ &  &  & 95.38 &  & &  &  \\
				\hline
				
				\multirow{9}{*}{90\% Sym. noise} & FixMatch (Retrain) &  &  &  & &  &  &  \\
				& DivideMix \cite{li2020dividemix} &  &  &  & 76.0 &  &  &  \\ 
                & DivideMix+ \cite{li2020dividemix} (Retrain) &  &  &  &  &  &  &  \\ \cline{2-9}
                
                & Alg. 2, Warmup stage: APL Loss ({\color{blue}{{Ours}}}) &  &  & 56.49 & &  &  &  \\
	            & Alg. 2, Warmup stage -APL + FixMatch  (Ours) &  &  & 79.73 &  & &  &  \\ \cline{2-9}

	            & Alg. 3, Student-Teacher Model (Ours), $L_{{lab}_{APL}} + L_{{un-weak}_{APL}}$ &  &  &  &  & &  &  \\
            
	            & Alg. 3, Student-Teacher Model (Ours), $L_{{lab}_{APL}} + L_{{un-weak}_{CE}}$ &  &  & &  & &  &  \\
	            & Alg. 3, Student-Teacher Model (Ours), $L_{{lab}_{APL}} + L_{{(un-(weak, strong) > \tau)}_{APL}} $ &  &  & 80.52 &  & &  &  \\
	            & Alg. 3, Student-Teacher Model (Ours), $L_{{lab}_{APL}} + L_{{(un-(weak, strong) > \tau)}_{APL}} + 0.1 * L_{{(un-(weak, strong) < \tau)}_{neg-ce}}$ &  &  & 81.23 &  & &  &  \\
				\hline
				
                \multirow{9}{*}{40\% Asym. noise} & FixMatch (Retrain) &  &  &  & &  &  &  \\
				& DivideMix \cite{li2020dividemix} &  &  &  & 93.4 &  &  &  \\ 
                & DivideMix+ \cite{li2020dividemix} (Retrain) &  &  &  &  &  &  &  \\ \cline{2-9}
                
                & Alg. 2, Warmup stage: APL Loss ({\color{blue}{{Ours}}}) &  &  &  & &  &  &  \\
	            & Alg. 2, Warmup stage -APL + FixMatch  (Ours) &  &  & 94.03 &  & &  &  \\ \cline{2-9}

	            & Alg. 3, Student-Teacher Model (Ours), $L_{{lab}_{APL}} + L_{{un-weak}_{APL}}$ &  &  &  &  & &  &  \\
            
	            & Alg. 3, Student-Teacher Model (Ours), $L_{{lab}_{APL}} + L_{{un-weak}_{CE}}$ &  &  & &  & &  &  \\
	            & Alg. 3, Student-Teacher Model (Ours), $L_{{lab}_{APL}} + L_{{(un-(weak, strong) > \tau)}_{APL}} $ &  &  &  &  & &  &  \\
	            & Alg. 3, Student-Teacher Model (Ours), $L_{{lab}_{APL}} + L_{{(un-(weak, strong) > \tau)}_{APL}} + 0.1 * L_{{(un-(weak, strong) < \tau)}_{neg-ce}}$ &  &  &  &  & &  &  \\
				\hline
\end{tabular}}
\caption{Performance comparison with SOTA Semi-Supervised Learning methods on CIFAR 10/100.}
\label{table:sota_ssl}
\end{table*}

\begin{table*}[t]

% 	\begin{center}
		
		\resizebox{1.0\textwidth}{!}{
			\begin{tabular}{|l | c c c c c |}
				\hline
				Datasets & \multicolumn{5}{c|}{Clothing1M} \\
				\hline
				\#Labels &40 & 250 & 4000 & 8000 & All Labels  \\ 
				\hline
                FixMatch \cite{sohn2020fixmatch} &  &  &  &- & \\ 
                Cross-Entropy &  &  &  &   &  69.21 \\ 
                
                DivideMix \cite{li2020dividemix} &  &  &  &   & 74.76 \\ \hline
                FixMatch (Retrain) &  &  &   &  & \\
                DivideMix + \cite{li2020dividemix} (Retrain) &  &  &  &   & \\ \hline
                
                Alg. 2, Warmup stage: SCE Loss ({\color{blue}{{Ours}}}) &  &  &  & 66.24 &  \\
	            Alg. 2, Warmup stage -SCE + FixMatch  (Ours) &  &  &  & 70.25* & \\ \hline

	            Alg. 3, Student-Teacher Model (Ours), $L_{{lab}_{APL}} + L_{{un-weak}_{APL}}$ &  &  &  & &   \\
	            
	            Alg. 3, Student-Teacher Model (Ours), $L_{{lab}_{APL}} + L_{{un-weak}_{CE}}$ &  &  &  &    &\\
	            Alg. 3, Student-Teacher Model (Ours), $L_{{lab}_{APL}} + L_{{(un-(weak, strong) > \tau)}_{CE}} $ &  &  &  &  &  \\
	            Alg. 3, Student-Teacher Model (Ours), $L_{{lab}_{APL}} + L_{{(un-(weak, strong) > \tau)}_{CE}} + L_{{(un-(weak, strong) < \tau)}_{MSE}}$ &  &  &  &  &  \\
				\hline

\end{tabular}}
\caption{Performance comparison with SOTA Semi-Supervised Learning methods on Clothing1M dataset.}
\label{table:sota_ssl}
\end{table*}

\begin{table*}

% 	\begin{center}
		
		\resizebox{\textwidth}{!}{
			\begin{tabular}{|l|c c c  c  c |  c c  c  c  c |}
				\hline
				Datasets & \multicolumn{5}{c|}{CIFAR-10} &\multicolumn{5}{c|}{CIFAR-100} \\
				\hline
				Noise Type & \multicolumn{4}{c|}{Sym.} & Asym. & \multicolumn{4}{c|}{Sym.} & Asym. \\ 
				\hline
				Methods/Noise Ratio & 20\% & 50\% & 80\%  & 90\% &   40\%  & 20\% & 50\% & 80\%  & 90\% &   40\% \\
				\hline\hline 
				
				DivideMix \cite{li2020dividemix} & \textbf{96.1} & \textbf{94.6} & \textbf{93.2} & \textbf{76.0} & \textbf{79.59} & \textbf{77.3} & \textbf{74.6} & \textbf{60.2 }& \textbf{31.5} & - \\
				APL-Loss, best \cite{ma2020normalized} & 89.22 & 86.05/0.4 & 79.78/0.6 & 52.71/0.8 & 79.59 & 65.31 & 59.48/0.4 & 48.06/0.6 & 25.80/0.8 & 47.22 \\ \hline
				
				Alg. 2, Warmup stage: APL Loss ({\color{blue}{{Ours}}}) &  &  &  & 52.77 &  & & & &  &  \\
				Alg. 2, Warmup stage-APL + FixMatch ({\color{blue}{{Ours}}}) &  &  &  & 70.71 &  & & & &  &  \\

				\hline

\end{tabular}}
\caption{Performance comparison with SOTA methods on learning with noisy labels.}
\label{table:sota_noisy}
\end{table*}

\begin{table*}[t]

% 	\begin{center}
		
		\resizebox{1.0\textwidth}{!}{
			\begin{tabular}{|l | c c c c c c c|}
				\hline
				Datasets & \multicolumn{7}{c|}{CIFAR10} \\
				\hline
				Hyper-parameters & Warmup epoch & LR & optimizer & weight decay & APL Loss & alpha-APL & beta-APL\\ 
				\hline
                FixMatch \cite{sohn2020fixmatch} &  &  &  &- \\ \hline
                FixMatch (Retrain) &  &  &   & \\
                DivideMix \cite{li2020dividemix} (Retrain) &  &  &  &   \\ \hline
                
                Alg. 2, Warmup stage: APL Loss ({\color{blue}{{Ours}}}) &  &  &  &  \\
	            Alg. 2, Warmup stage -APL + FixMatch  (Ours) &  &  &  &   \\ \hline

	            Alg. 3, Student-Teacher Model (Ours), $L_{{lab}_{APL}} + L_{{un-weak}_{APL}}$ &  &  &  &    \\
	            
	            Alg. 3, Student-Teacher Model (Ours), $L_{{lab}_{APL}} + L_{{un-weak}_{CE}}$ &  &  &  &    \\
	            Alg. 3, Student-Teacher Model (Ours), $L_{{lab}_{APL}} + L_{{(un-(weak, strong) > \tau)}_{CE}} $ &  &  &  &    \\
	            Alg. 3, Student-Teacher Model (Ours), $L_{{lab}_{APL}} + L_{{(un-(weak, strong) > \tau)}_{CE}} + L_{{(un-(weak, strong) < \tau)}_{MSE}}$ &  &  &  &    \\
				\hline

\end{tabular}}
\caption{Performance comparison with SOTA Semi-Supervised Learning methods on Clothing1M dataset.}
\label{table:sota_ssl}
\end{table*}
